# Supplementary material for: Generative Adversarial Imagination for Sample Efficient Deep Reinforcement Learning
Source: arXiv:1904.13255 source file (2019-06-10)
Supplement: Supplementary file 1 [file submission.tex]

The submitted zip file contains:
\begin{itemize}
    \item Figures used throughout the thesis (directory: \textbf{figures})
    \item Copy of the thesis (file: \textbf{kxk633\_kielak\_thesis.pdf})
    \item Sample research logs used for optimising hyperparameters (directory: \textbf{research\_logs})
    \item The Git repository address (file: git\_repository.txt)
    \item Source code (directory: \textbf{gairl})
\end{itemize}

The source code is structured as follows:
\begin{itemize}
    \item \textbf{requirements.txt} specifies required Python libraries.
    \item \textbf{resources} contains MNIST dataset used to debug and optimise generative models.
    \item \textbf{gairl} consists of the actual functional source code.
    \item \textbf{tests} includes unit tests for most critical and bug-prone parts of the code.
    \item \textbf{README.md} provides more detailed description of the code and how to successfully perform experiments.
\end{itemize}

Python3.6, together with libraries specified in the \textbf{requirements.txt} file, is a requirement. Additionally, Open AI Gym (included in the \textbf{requirements.txt}) may need \texttt{swig} and \texttt{python-opengl} packages (to install on Ubuntu\textgreater=16.04: \linebreak \texttt{sudo apt-get install -y swig python-opengl}). To properly run the code \texttt{PYTHONPATH} should point to the first level \textbf{gairl} directory.

Experiments can be executed by running one out of entry-points in the \linebreak \textbf{gairl/experiments} package. High-level configuration for the experiment can be set in the \textbf{gairl/config.py} file. Then, algorithm's (hyper)parameters can be changed in the appropriate algorithm-specific configuration file.

Additionally, the Git repository contains TensorBoard summaries of selected, previously performed experiments in its Git-LFS system (warning: they may take up to 7GB of space). Refer to the TensorBoard documentation on how to open the summaries. Moreover, commits history provides good overview of the implementation and experimentation progress (second term only, the first one was focused on reading and theoretical research).
